# Supplementary material for: Anomalous circularly polarized light emission in organic light-emitting diodes caused by orbital-momentum locking
Source: arXiv:2205.09099 source file (2022-12-18)
Supplement: Supplementary file 1 [file SI.pdf]

**Supplementary Information**


Table S1 Summary of reported $g_{PL}$ and $g_{EL}$.

Scheme S1 Molecular structures of materials in Fig. 2 analysis.

Figure S1 Absorption and circular dichroism spectra.

Figure S2 PL and absorption dissymmetry factor measured from opposite direction.

Figure S3 Detailed CP-EL spectra of semi-transparent inverted CP-OLEDs.

Figure S4 Detailed CP-EL spectra of semi-transparent conventional CP-OLEDs.

Figure S5: 2D GIWAXS profile of chiral F8BT:aza[6]H films casted on different substrates.

Figure S6: EL spectra of F8BT:aza[6]H blend measured from different OLED structures with interlayers.

Figure S7 $g_{\mathrm{EL}}$ as a function of active layer thickness.

Figure S8 Detailed CP-EL spectra of inverted CP-OLEDs with different reflective electrode.

Section S1 Electric and Magnetic Dipoles in Plane-Wave Basis

Section S2 CP and Orbital Angular Momentum (OAM)

Figure S9: Illustration of a band structure with orbital polarization.

Section S3 Intrinsic Momentum and Mobility-related Drift Velocity.

Table S1: Summary of reported $g_{\mathrm{PL}}$ and $g_{\mathrm{EL}}$.

| Emissive layer | Category | $\lvert g_{\mathrm{PL}}\rvert$ | $\lvert g_{\mathrm{EL}}\rvert$ | Comment |
|---|---|---|---|---|
| F8BT[1] | Polyfluorene | 0.21 | 0.65 | |
| F8BT[2] | Polyfluorene | 0.21 | 0.48 | |
| PFO crystalline[3] | Polyfluorene | 0.21 | 0.42 | |
| PFO beta-phase[3] | Polyfluorene | 0.39 | 0.44 | |
| CsEu((-)hfbc)$_4$[4] | Lanthanide complex | 1.21 | 0.15 | Used for Figure 2b analysis |
| $M$-Pt[5] | Phosphorescent | $4.9\times10^{-3}$ | $1.1\times10^{-3}$ | Used for Figure 2b analysis |
| $\Delta$-$fac$-Ir(ppy)$_3$[6] | Phosphorescent | $3.15\times10^{-3}$ | $2.8\times10^{-4}$ | |
| $\Delta$-Ir(ppy)$_2$(acac)[6] | Phosphorescent | $1.33\times10^{-3}$ | $3.1\times10^{-4}$ | |
| $\Delta$-(tfpqz)$_2$Ir($R$-L$_2$)[7] | Phosphorescent | $9\times10^{-4}$ | $5\times10^{-4}$ | |
| $\Delta$-Ir(dfppy)$_2$($S$-sdpp)[8] | Phosphorescent | $1.7\times10^{-3}$ | $2.1\times10^{-3}$ | |
| $\Delta$-Ir(dfppy)$_2$($R$-sdpp)[8] | Phosphorescent | $1.2\times10^{-3}$ | $2.1\times10^{-3}$ | |
| $P$-Pt[9] | Phosphorescent | $4\times10^{-3}$ | $1.3\times10^{-3}$ | |
| ($R$)-BN-CF[10] | TADF | $1.2\times10^{-3}$ | $2.1\times10^{-3}$ | |
| ($S$)-CPDCz[11] | TADF | $3.7\times10^{-4}$ | $5.5\times10^{-4}$ | |
| ($S$)-CPDCB[11] | TADF | $5.8\times10^{-4}$ | $8.6\times10^{-4}$ | |
| ($R$)-OBN-DPA[12] | TADF | $2.52\times10^{-3}$ | $2.3\times10^{-3}$ | |
| ($R$)-OBN-Cz[13] | TADF | $1.4\times10^{-3}$ | $2.3\times10^{-3}$ | |
| ($R$)-ODQPXZ[14] | TADF | $4.6\times10^{-4}$ | $6.0\times10^{-4}$ | |

| | | | |
|---|---|---|---|
| (S)-SFST[15] | TADF | $4\times10^{-3}$ | $1.3\times10^{-3}$ |
| $(S,S)$-CPAD[16] | TADF | $2.5\times10^{-3}$ | $1.8\times10^{-3}$ |
| $(S,S)$-CAI-Cz[17] | TADF | $1.1\times10^{-3}$ | $1.7\times10^{-3}$ |

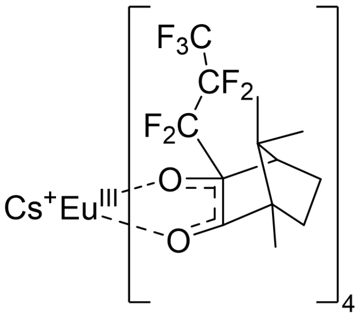


CsEu((-)hfbc)$_4$

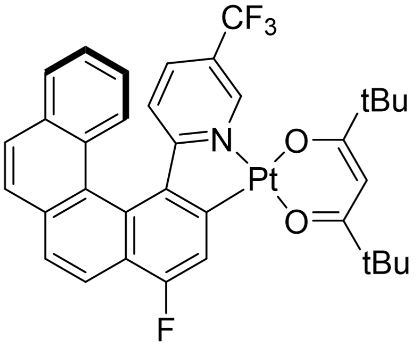


*M*-Pt

Scheme S1: Molecular structures of CsEu((-)hfbc)$_4$ and $M$-Pt for Figure 2 analysis

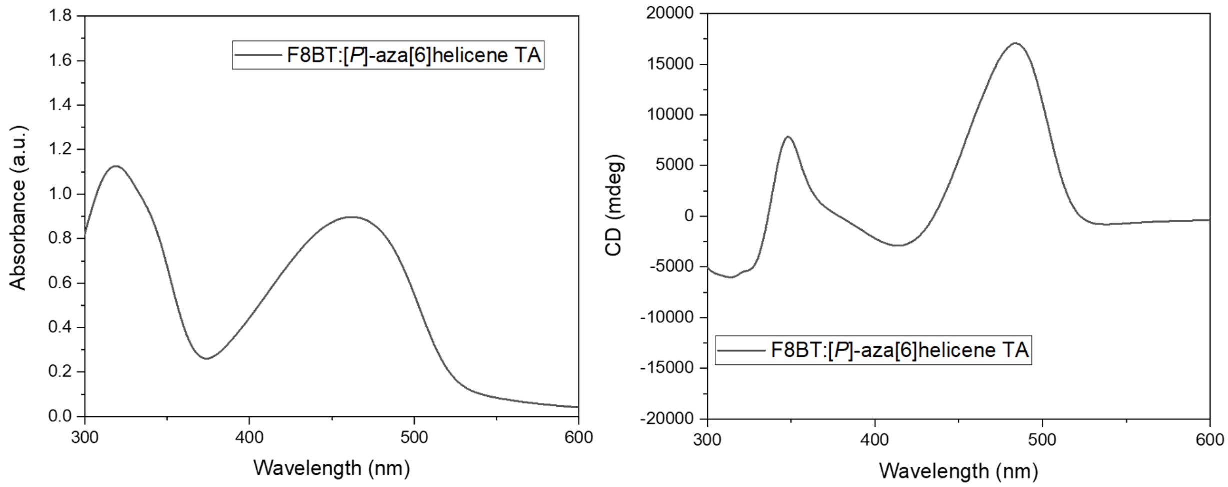


Figure S1: Absorption (left) and circular dichroism (right) spectra of F8BT:[P]-aza[6]helicene thermally annealed (TA) films

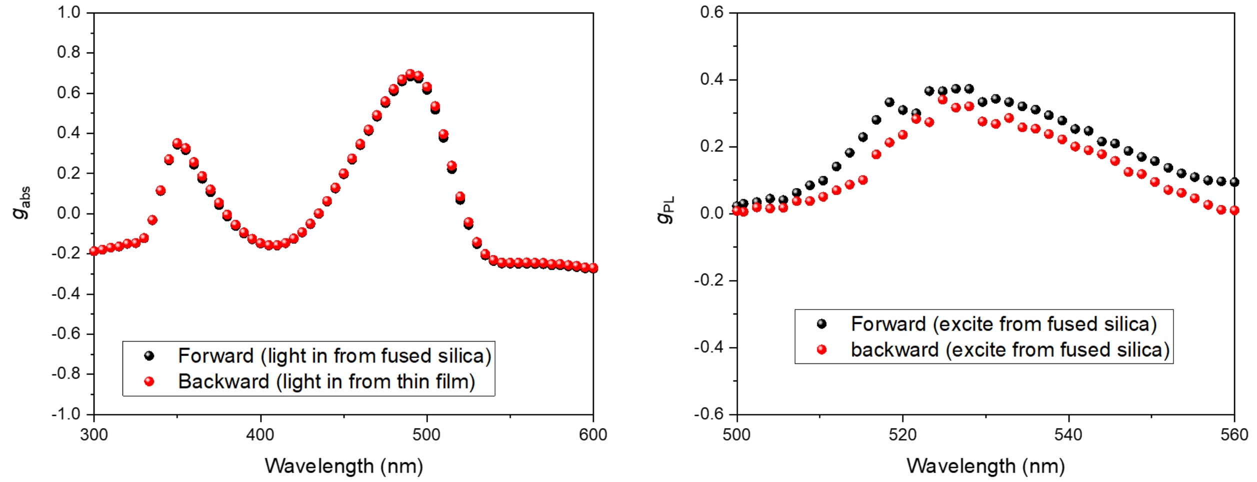


Figure S2: $g_{abs}$ (left) and $g_{PL}$ (right) spectra of F8BT:[P]-aza[6]helicene thermally annealed (TA) films measured from opposite direction.

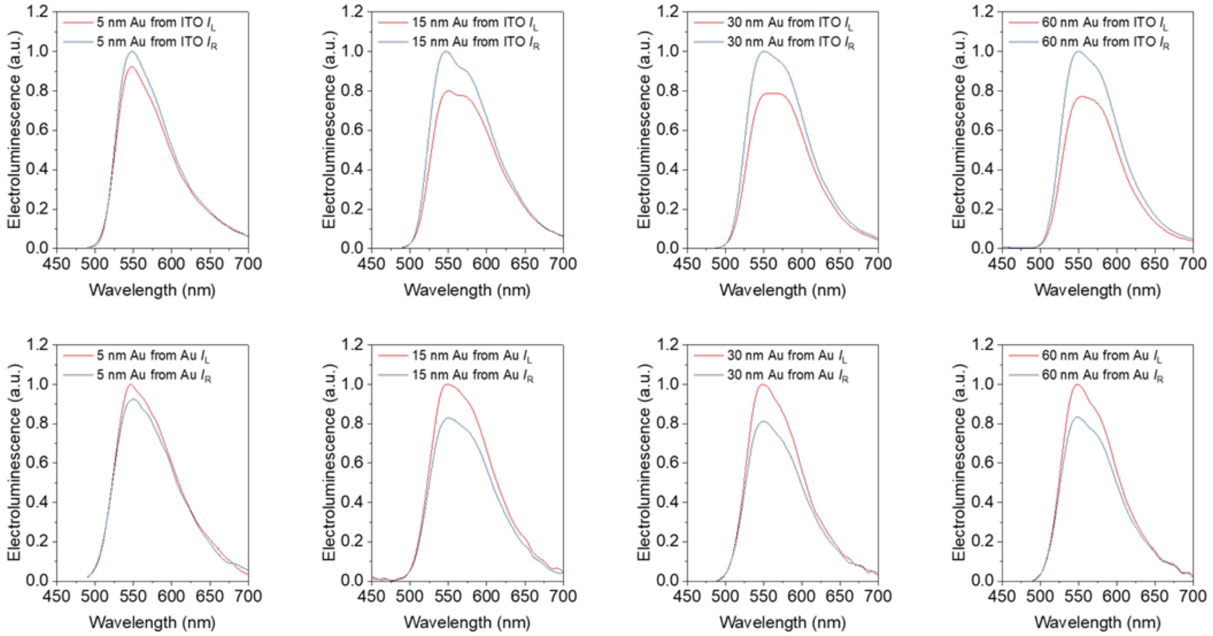


Figure S3: Detailed CP-EL spectra of semi-transparent inverted CP-OLEDs. Device structure: ITO/ZnO/PEIE/ F8BT:[P]-aza[6]helicene/TCTA/MoOx/Au (x nm)

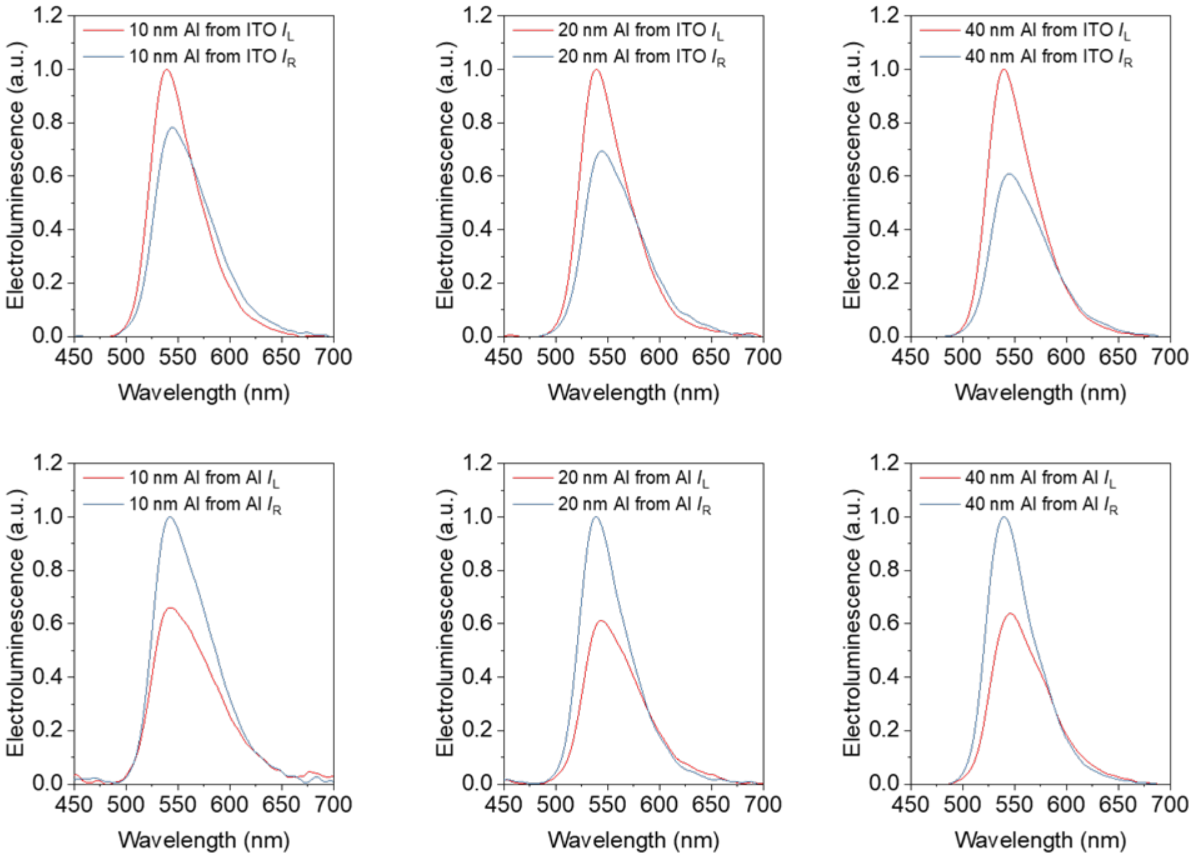


Figure S4: Detailed CP-EL spectra of semi-transparent conventional CP-OLEDs. ITO/PEDOT:PSS/TFB/ F8BT:[P]-aza[6]helicene/TPBi/Ca/Al (x nm)

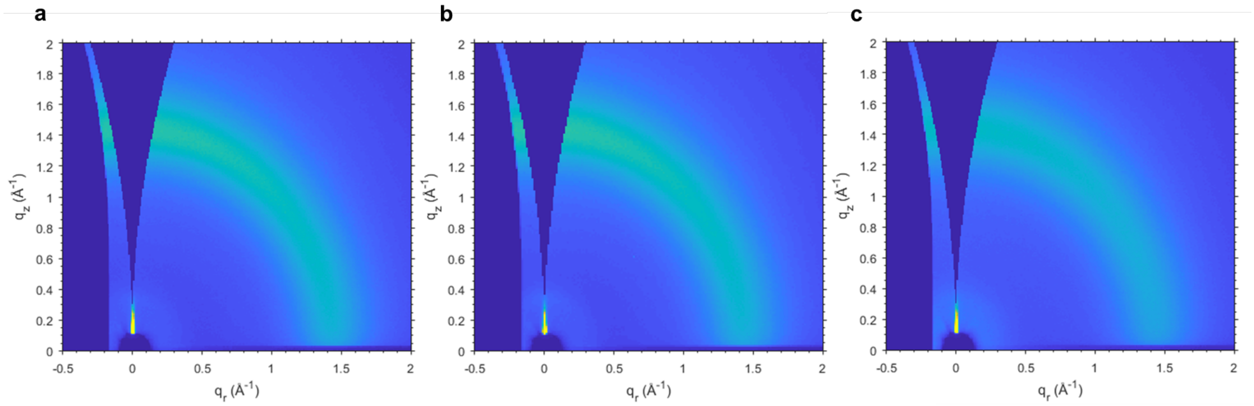


Figure S5: 2D GIWAXS profile of chiral F8BT:aza[6]H films casted on (a) ITO/PEDOT:PSS/TFB (b) ITO/ZnO/PEIE, and (c) on cleaned fused silica. No apparent morphological changes can be observed from films casted on different substrates.

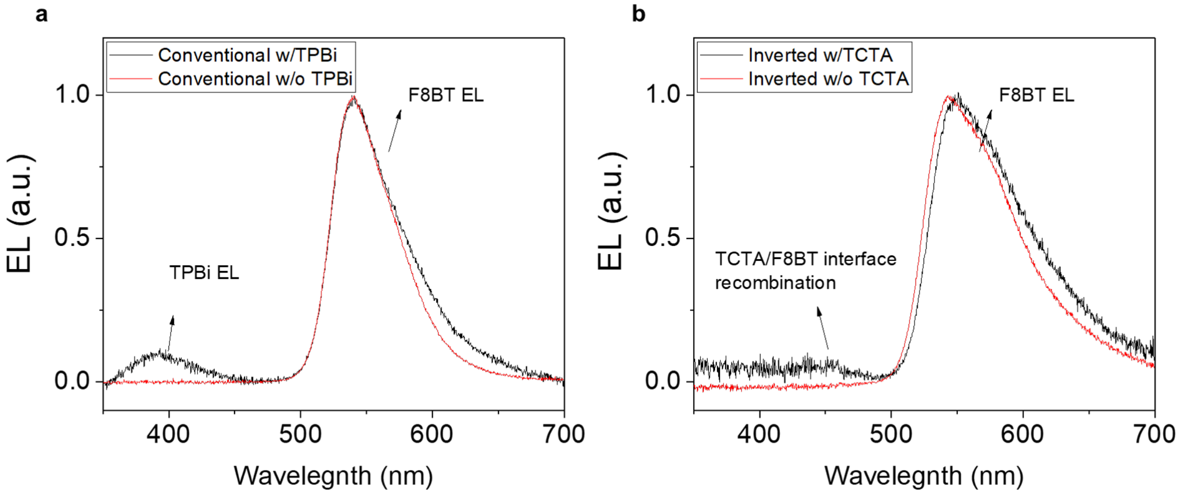


Figure S6: EL profiles of F8BT:aza[6]H blend measured from different OLED structures. (a) conventional OLED (ITO injects holes) with/without ETL TPBi, (b) inverted OLED (ITO injects electrons) with/without HTL (TCTA). The appearance of the TPBi peak and TCTA/F8BT surface recombination indicate that the recombination zone in both devices are pinned at the far interface of F8BT, away from ITO electrode.

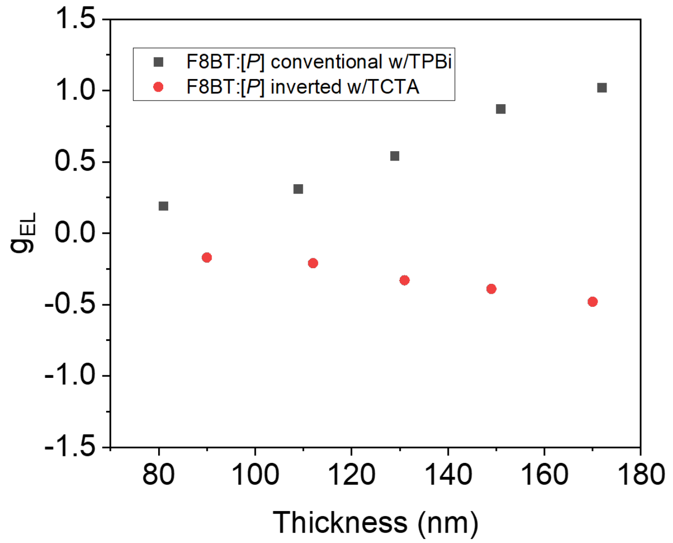


Figure S7: $g_{EL}$ as a function of active layer thickness. Thicknesses were controlled via different spin-speed. Conventional device (ITO injects holes) ITO/PEDOT:PSS/TFB/ F8BT:[P]-aza[6]helicene/TPBi/Ca/Al. Inverted device (ITO injects electrons) : ITO/ZnO/PEIE/ F8BT:[P]-aza[6]helicene/TCTA/MoOx/Au

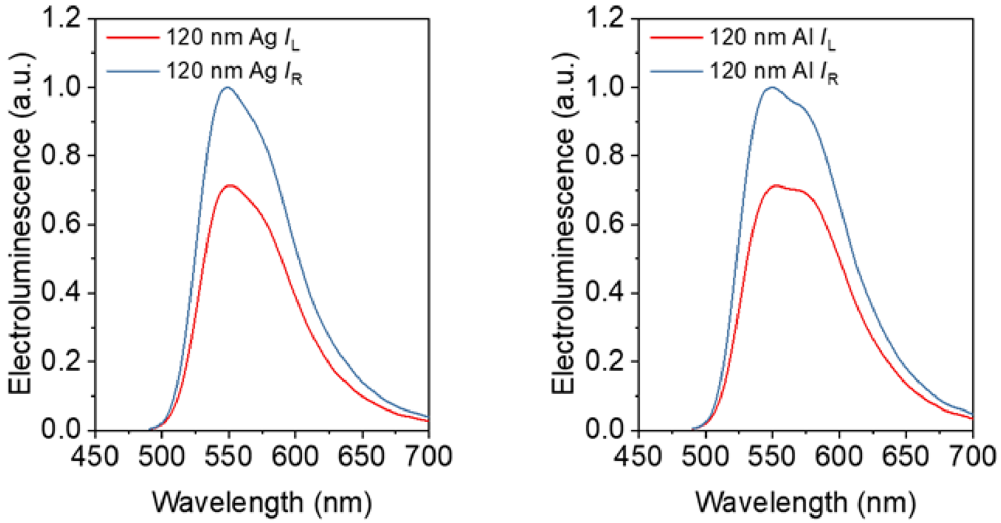


Figure S8: Detailed CP-EL spectra of inverted CP-OLEDs with different reflective electrode. ITO/ZnO/PEIE/ F8BT:[P]-aza[6]helicene/TCTA/MoOx/Ag (or Al) (120 nm)

## S1 Electric and Magnetic Dipoles in Plane-Wave Basis

In this section we explicitly derive the expressions of electric and magnetic transition dipoles in terms of the coefficients of plane-wave basis. Tha wavefunctions of HOMO/LUMO, *i.e.* $\psi_{0,1}$ can be expanded in the series of plane-wave functions as:

$$\begin{aligned}
|0,1\rangle &= \sum_{\boldsymbol{G}} c_{\boldsymbol{G}}^{0,1} e^{i\boldsymbol{G}\cdot\boldsymbol{r}} = |0^0,1^0\rangle + |0^+,1^+\rangle + |0^-,1^-\rangle\,, \\
|0^0,1^0\rangle &= \sum_{\boldsymbol{G}} c_{\boldsymbol{G}}^{0,1} e^{i\boldsymbol{G}\cdot\boldsymbol{r}}\Big|_{G_z=0} = \sum_{\boldsymbol{G}}^{0} c_{\boldsymbol{G}}^{0,1} e^{i\boldsymbol{G}\cdot\boldsymbol{r}}, \\
|0^+,1^+\rangle &= \sum_{\boldsymbol{G}} c_{\boldsymbol{G}}^{0,1} e^{i\boldsymbol{G}\cdot\boldsymbol{r}}\Big|_{G_z>0} = \sum_{\boldsymbol{G}}^{+} c_{\boldsymbol{G}}^{0,1} e^{i\boldsymbol{G}\cdot\boldsymbol{r}}, \\
|0^-,1^-\rangle &= \sum_{\boldsymbol{G}} c_{\boldsymbol{G}}^{0,1} e^{i\boldsymbol{G}\cdot\boldsymbol{r}}\Big|_{G_z<0} = \sum_{\boldsymbol{G}}^{-} c_{\boldsymbol{G}}^{0,1} e^{i\boldsymbol{G}\cdot\boldsymbol{r}}.
\end{aligned} \tag{S1}$$

The electric dipole $\langle 0^+|r_\alpha|1^+\rangle$ can be derived as:

$$\begin{aligned}
\langle 0^+|r_\alpha|1^+\rangle &= \int d\boldsymbol{r}\ (\psi_0^+)^* r_\alpha \psi_1^+ \\
&= \int d\boldsymbol{r}\ \sum_{\boldsymbol{G}'}^{+}\sum_{\boldsymbol{G}}^{+} (c_{\boldsymbol{G}'}^0)^* r_\alpha c_{\boldsymbol{G}}^1 e^{i(\boldsymbol{G}-\boldsymbol{G}')\cdot\boldsymbol{r}} \\
&= \sum_{\boldsymbol{G}'}^{+}\sum_{\boldsymbol{G}}^{+} (c_{\boldsymbol{G}'}^0) c_{\boldsymbol{G}}^1 \left(i\frac{\partial}{\partial G_\alpha}\right) \int d\boldsymbol{r}\ e^{i(\boldsymbol{G}-\boldsymbol{G}')\cdot\boldsymbol{r}} \\
&= -i(2\pi)^3 \sum_{\boldsymbol{G}'}^{+}\sum_{\boldsymbol{G}}^{+} (c_{\boldsymbol{G}'}^0) c_{\boldsymbol{G}}^1 \frac{\partial\delta(\boldsymbol{G}-\boldsymbol{G}')}{\partial G_\alpha} \\
&= -i(2\pi)^3 \sum_{\boldsymbol{G}}^{+} c_{\boldsymbol{G}}^1 \left(\frac{\partial c_{\boldsymbol{G}}^0}{\partial G_\alpha}\right),
\end{aligned} \tag{S2}$$

where two identities

$$\begin{aligned}
\int d\boldsymbol{r}\ e^{i(\boldsymbol{G}-\boldsymbol{G}')\cdot\boldsymbol{r}} &= (2\pi)^3\delta(\boldsymbol{G}-\boldsymbol{G}'), \\
\sum_{\boldsymbol{G}'} f(\boldsymbol{G}')\frac{\partial\delta(\boldsymbol{G}-\boldsymbol{G}')}{\partial\lambda} &= \frac{\partial f(\boldsymbol{G})}{\partial\lambda},
\end{aligned} \tag{S3}$$

have been used. The magnetic dipole $\langle 0^+|m_\alpha|1^+\rangle$ can be similarly derived as:

$$\begin{aligned}\langle 0^+|m_\alpha|1^+\rangle &= \frac{e}{2m_e}\langle 0^+|L_\alpha|1^+\rangle \\ &= \frac{e\hbar}{2m_e}\sum_{\boldsymbol{G}'}^{+}\sum_{\boldsymbol{G}}^{+}(c^0_{\boldsymbol{G}'})^* c^1_{\boldsymbol{G}}\left(G_y\frac{\partial}{\partial G_x} - G_x\frac{\partial}{\partial G_y}\right)\int d\boldsymbol{r}\ e^{i(\boldsymbol{G}-\boldsymbol{G}')\cdot\boldsymbol{r}} \\ &= -i\frac{(2\pi)^3 e\hbar}{2m_e}\sum_{\boldsymbol{G}}^{+} c^1_{\boldsymbol{G}}\left(G_y\frac{\partial c^0_{\boldsymbol{G}}}{\partial G_x} - G_x\frac{c^0_{\boldsymbol{G}}}{\partial G_y}\right)^*.\end{aligned} \tag{S4}$$

The electric or magnetic dipole itself depends on the gauge choice of $|0\rangle$ and $|1\rangle$ but the products $x^{01}y^{10}$ and $\boldsymbol{r}^{01}\cdot\boldsymbol{m}^{10}$ is gauge independent.

## S2 CP and Orbital Angular Momentum (OAM)

In this section we relate the CP to an OAM-like quantity. The intensity defference between (right- and left- handed) circularly polarized light can be rewritten as:

$$\begin{aligned}I_L - I_R &= -\frac{2\pi e^2}{\hbar}\mathrm{Im}\,[x^{01}y^{10}]\delta(\varepsilon_1-\varepsilon_0-\hbar\omega) \\ &= i\frac{\pi e^2}{\hbar}[\langle 0|\,x\,|1\rangle\,\langle 1|\,y\,|0\rangle - (x\leftrightarrow y)]\delta(\varepsilon_1-\varepsilon_0-\hbar\omega) \\ &= i\frac{\pi e^2}{\hbar}\left[\langle 0|\,x\,|1\rangle\,\frac{-i\hbar\,\langle 1|\,p_y\,|0\rangle}{m_e(\varepsilon_1-\varepsilon_0)} - (x\leftrightarrow y)\right]\delta(\varepsilon_1-\varepsilon_0-\hbar\omega) \\ &= \frac{\pi e^2}{m_e\hbar\omega}\langle L^1_z\rangle_0\delta(\varepsilon_1-\varepsilon_0-\hbar\omega)\end{aligned} \tag{S5}$$

where $\langle L^1_z\rangle_0 = \langle 0|\,x\,|1\rangle\,\langle 1|\,p_y\,|0\rangle - \langle 0|\,y\,|1\rangle\,\langle 1|\,p_x\,|0\rangle$ is an OAM-like variable and $\langle\cdots\rangle_0$ means the expectation value at state $|0\rangle$. It should be noted that Eq. (S5) is a gauge-invariant form of CP-EL which is different from the gauge-dependent magnetic dipole $m^{01}_z$ or $m^{00}_z$ in Eq. (S4).

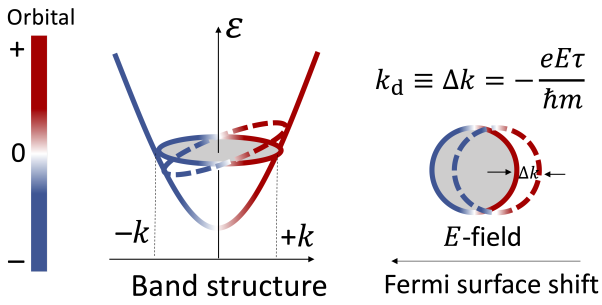


Figure S9: Illustration of a band structure with orbital polarization. In the presence of an E-field ($E$), the Fermi surface shifts. Here $\pm k$ is the intrinsic momentum in the band structure, and $k_d$ is the drift momentum induced by $\tau$ and E-field.

## S3 Intrinsic Momentum and Mobility-related Drift Velocity

In the context of orbital-momentum locking, we should clarify the definition of "momentum", which is different from the drift momentum ($k_d$) (or drift velocity) in transport. (i) For the orbital-momentum locking, we refer to the intrinsic orbital and intrinsic momentum ($k \approx \pm n\pi/d$, $d$ is the molecule size) inside the chiral molecule or the chiral aggregate. Here $k$ is proportional to the interatomic coupling that is a large value 0.1 or 1 eV. The induced orbital polarization can also be a large value for given $k$. In transport, electrons and holes with polarized orbitals meet and recombine with each other, to generate CPL. (ii) The drift momentum $k_d = -\frac{eE\tau}{\hbar m}$ comes from the electric field ($E$) acceleration between molecules/aggregates within a scattering time $\tau$. Because $\tau$ is small and $m$ is large for organic semiconductors, the mobility is usually low. If we borrow the band structure language (see the following Fig. S9), $k_d$ characterizes the Fermi surface shift and constrains the total number of free moving electrons/holes. However, the orbital of a moving electron is determined by the orbital polarization at $\pm k$ in the intrinsic band structure. In summary,

electrons have intrinsic spontaneous momentum and orbital inside the molecule. Although the low-mobility reduces the total amount of free electrons and holes in transport, it does not necessarily reduce the orbital polarization of existing carriers.

## References


1. Wan, L. *et al.* Inverting the handedness of circularly polarized luminescence from light-emitting polymers using film thickness. *ACS nano* **13**, 8099–8105 (2019).

2. Wan, L. *et al.* Highly efficient inverted circularly polarized organic light-emitting diodes. *ACS Applied Materials & Interfaces* **12**, 39471–39478 (2020).

3. Wan, L., Shi, X., Wade, J., Campbell, A. J. & Fuchter, M. J. Strongly circularly polarized crystalline and $\beta$-phase emission from poly (9, 9-dioctylfluorene)-based deep-blue light-emitting diodes. *Advanced Optical Materials* **9**, 2100066 (2021).

4. Zinna, F. *et al.* Design of lanthanide-based oleds with remarkable circularly polarized electroluminescence. *Advanced Functional Materials* **27**, 1603719 (2017).

5. Yan, Z. *et al.* Configurationally Stable Platinahelicene Enantiomers for Efficient Circularly Polarized Phosphorescent Organic Light-Emitting Diodes. *Chemistry – A European Journal* **25**, 5672–5676 (2019).

6. Li, T.-Y. *et al.* Circularly polarised phosphorescent photoluminescence and electroluminescence of iridium complexes. *Scientific Reports* **5**, 14912 (2015).

7. Yan, Z. P. *et al.* Chiral iridium(III) complexes with four-membered Ir-S-P-S chelating rings for high-performance circularly polarized OLEDs. *Chemical Communications* **55**, 8215–8218 (2019).

8. Lu, J. J. *et al.* Pyridinylphosphorothioate-based blue iridium(III) complex with double chiral centers for circularly polarized electroluminescence. *Journal of Materials Chemistry C* **9**, 5244–5249 (2021).

9. Yan, Z. P., Luo, X. F., Liao, K., Zheng, Y. X. & Zuo, J. L. Rational Design of the Platinahelicene Enantiomers for Deep-Red Circularly Polarized Organic Light-Emitting Diodes. *Frontiers in Chemistry* **8**, 501 (2020).

10. Song, F. *et al.* Highly Efficient Circularly Polarized Electroluminescence from Aggregation-Induced Emission Luminogens with Amplified Chirality and Delayed Fluorescence. *Advanced Functional Materials* **28**, 1800051 (2018).

11. Sun, S. *et al.* Thermally activated delayed fluorescence enantiomers for solution-processed circularly polarized electroluminescence. *Journal of Materials Chemistry C* **7**, 14511–14516 (2019).

12. Wu, Z. G. *et al.* Non-doped and doped circularly polarized organic light-emitting diodes with high performances based on chiral octahydro-binaphthyl delayed fluorescent luminophores. *Journal of Materials Chemistry C* **7**, 7045–7052 (2019).

13. Wu, Z. *et al.* Chiral Octahydro-Binaphthol Compound-Based Thermally Activated Delayed Fluorescence Materials for Circularly Polarized Electroluminescence with Superior EQE of 32.6% and Extremely Low Efficiency Roll-Off. *Advanced Materials* **31**, 1900524 (2019).

14. Xie, F.-M. *et al.* Efficient Circularly Polarized Electroluminescence from Chiral Thermally Activated Delayed Fluorescence Emitters Featuring Symmetrical and Rigid Coplanar Acceptors. *Advanced Optical Materials* **9**, 2100017 (2021).

15. Yang, S. Y. *et al.* Circularly Polarized Thermally Activated Delayed Fluorescence Emitters in Through-Space Charge Transfer on Asymmetric Spiro Skeletons. *Journal of the American Chemical Society* **142**, 17756–17765 (2020).

16. Li, M., Wang, M. Y., Wang, Y. F., Feng, L. & Chen, C. F. High-Efficiency Circularly Polarized Electroluminescence from TADF-Sensitized Fluorescent Enantiomers. *Angewandte Chemie International Edition* **60**, 20728–20733 (2021).

17. Li, M. *et al.* Stable Enantiomers Displaying Thermally Activated Delayed Fluorescence: Efficient OLEDs with Circularly Polarized Electroluminescence. *Angewandte Chemie International Edition* **57**, 2889–2893 (2018).
